# Supplementary material for: H2O-SDF: Two-phase Learning for 3D Indoor Reconstruction using Object Surface Fields
Source: arXiv:2402.08138 source file (2024-03-08)

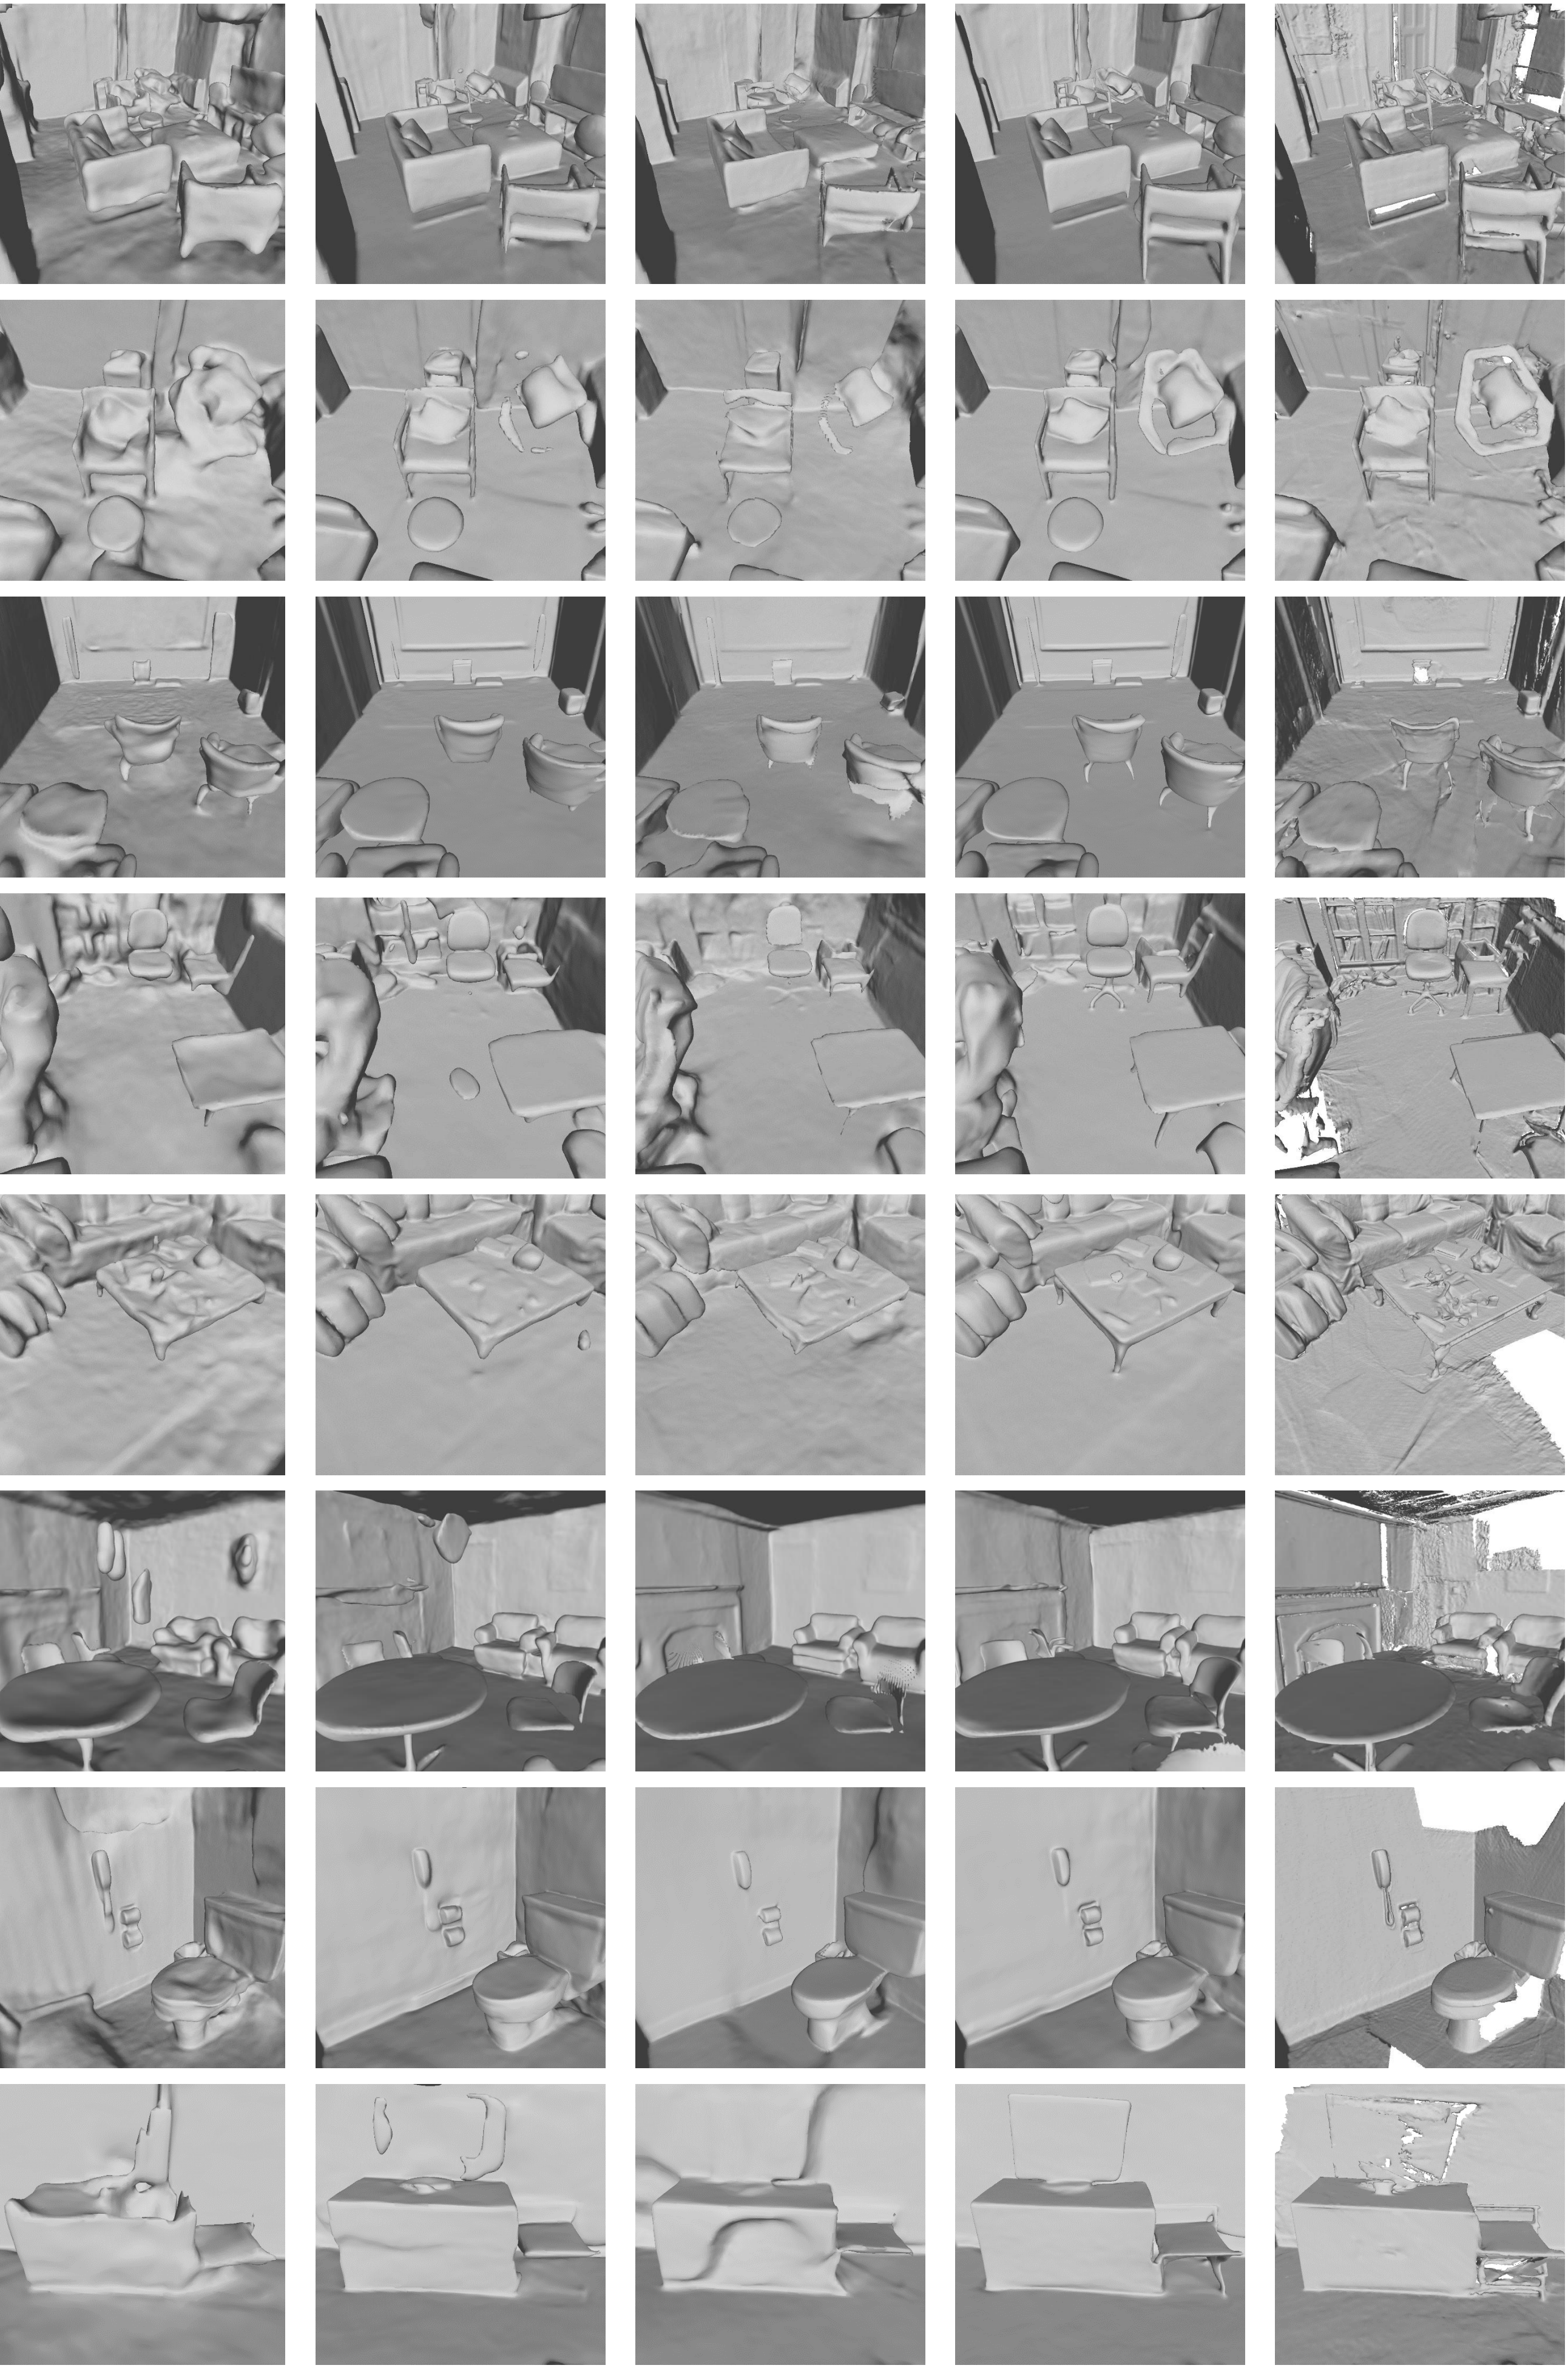



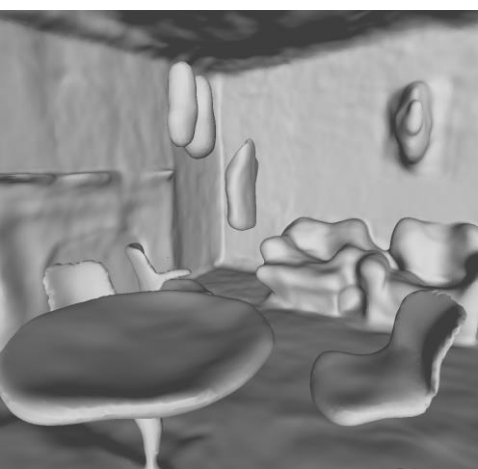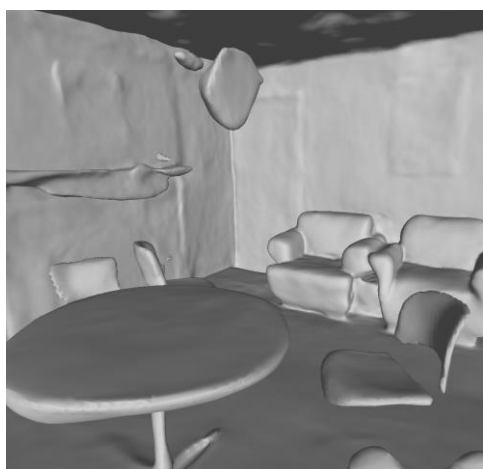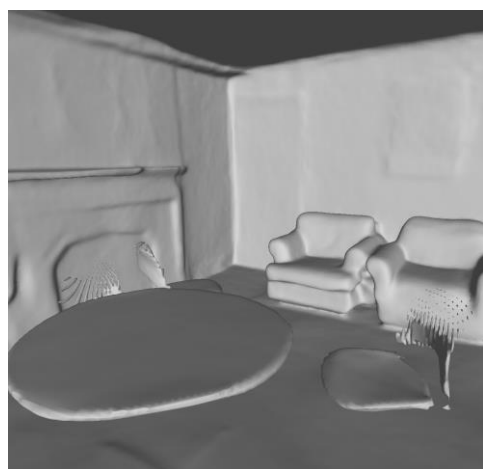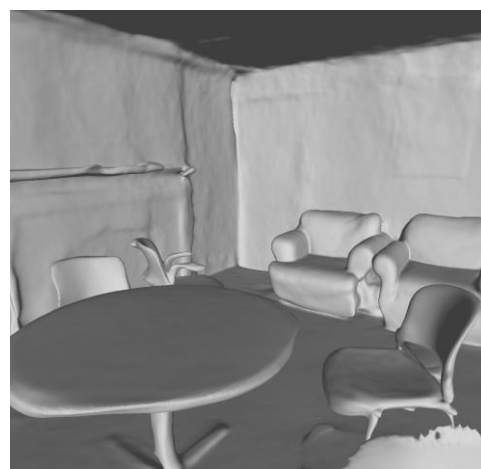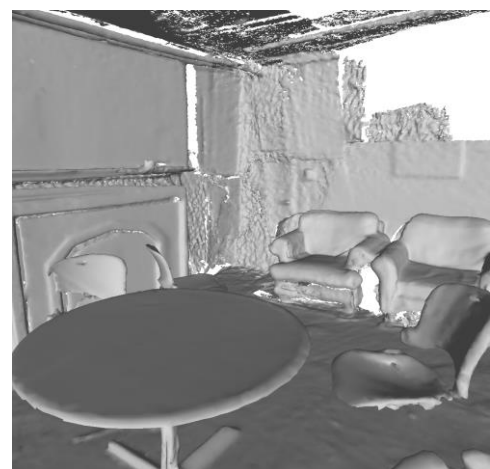

Supplement: Supplementary file 1 [file Supple_3d_recon.pdf]
