# Supplementary material for: H2O-SDF: Two-phase Learning for 3D Indoor Reconstruction using Object Surface Fields
Source: arXiv:2402.08138 source file (2024-03-08)
Supplement: Supplementary file 2 [file Supple_nvs.tex]

\begin{figure}[h]
    \centering
    \includegraphics[width=\textwidth]{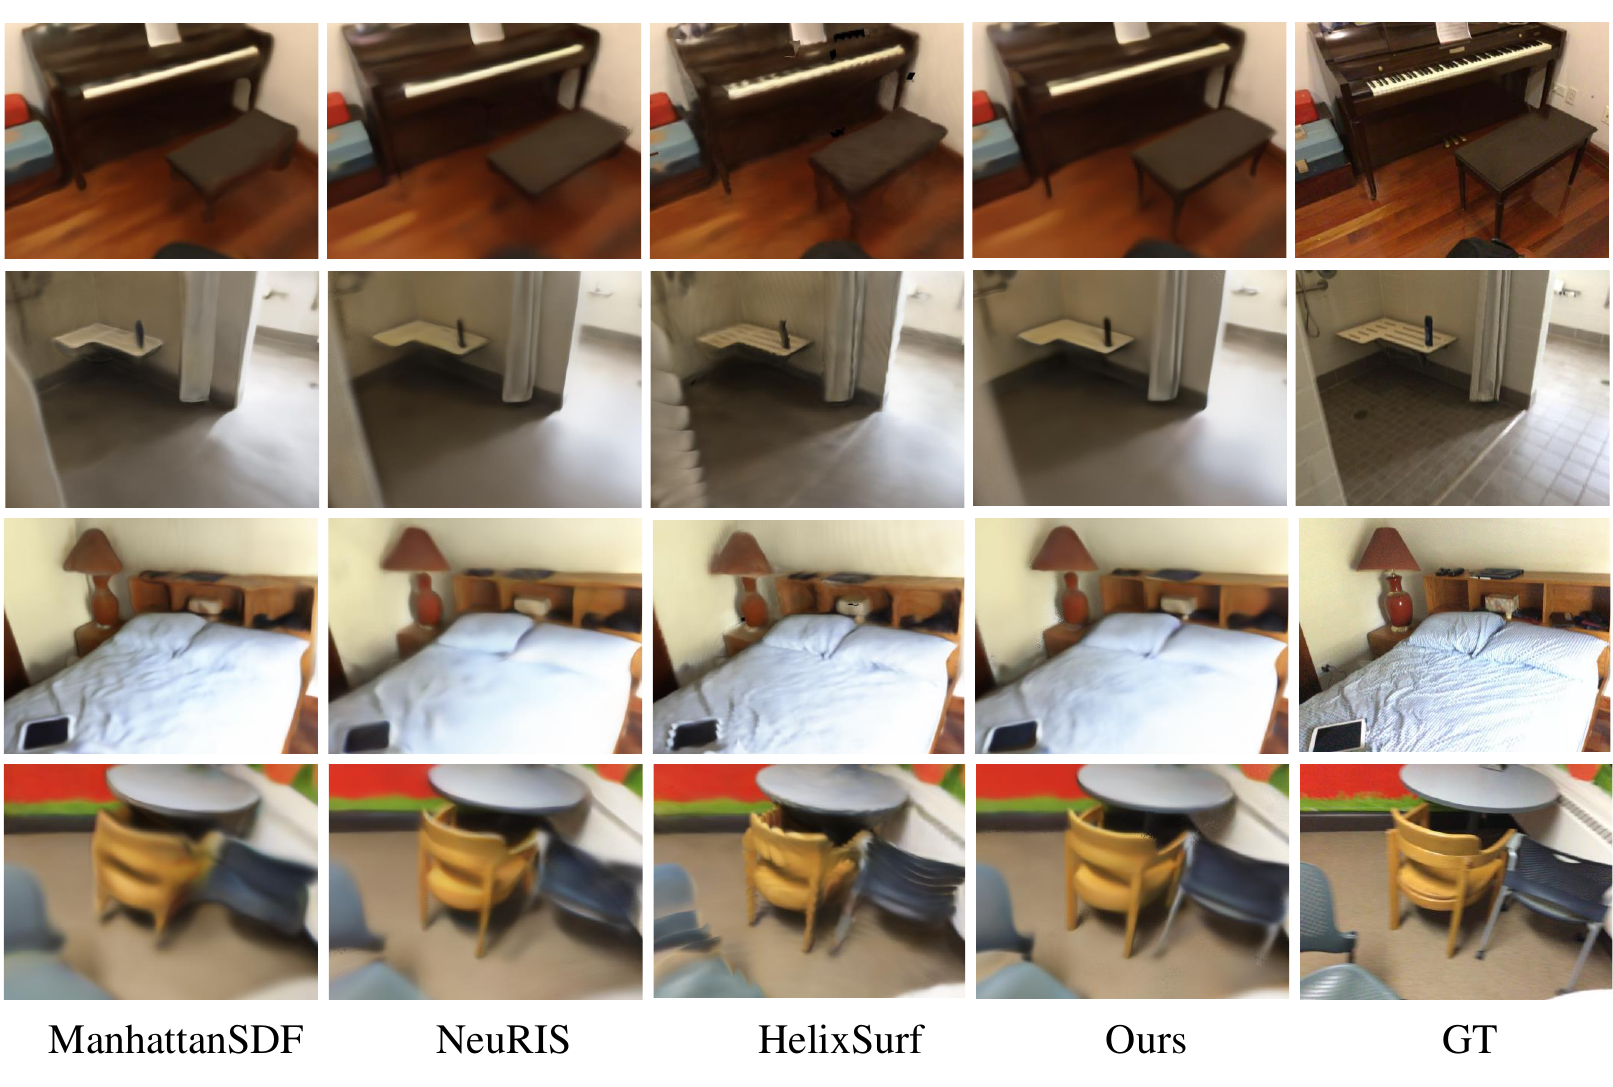}
    \caption{Novel view synthesis results.}
    \label{fig:supple_nvs}
\end{figure}
