# Supplementary material for: H2O-SDF: Two-phase Learning for 3D Indoor Reconstruction using Object Surface Fields
Source: arXiv:2402.08138 source file (2024-03-08)
Supplement: Supplementary file 3 [file supple_replica.tex]

% \begin{figure}
% % \includegraphics[trim=6cm 3.5cm 7cm 4.1cm, clip, width=\textwidth]{Figure/pdf/supple/supple_replica.pdf}

% \begin{minipage}{\textwidth}
%     \centering
%     \includegraphics[trim=6cm 2cm 6cm 2cm, clip, width=\textwidth]{Figure/pdf/supple/replica_result_birdview_v2.pdf}
%     \fontsize{10}{1}\selectfont
%     \vspace{-5pt}
%     \hspace{2.3cm} NeuRIS \hspace{3cm} Ours \hspace{3.3cm} Reference
% \end{minipage}
% \vspace{5pt}
% \caption{ \textbf{Evaluation on Replica dataset.}
% }\label{fig:supple_replica}
% % \vspace{-5pt}
% \end{figure}

\begin{figure}[h]
    % \centering
    \begin{tikzpicture}
        \node at (0,0) {\includegraphics[trim=6cm 2cm 6cm 2cm, clip, width=\textwidth]{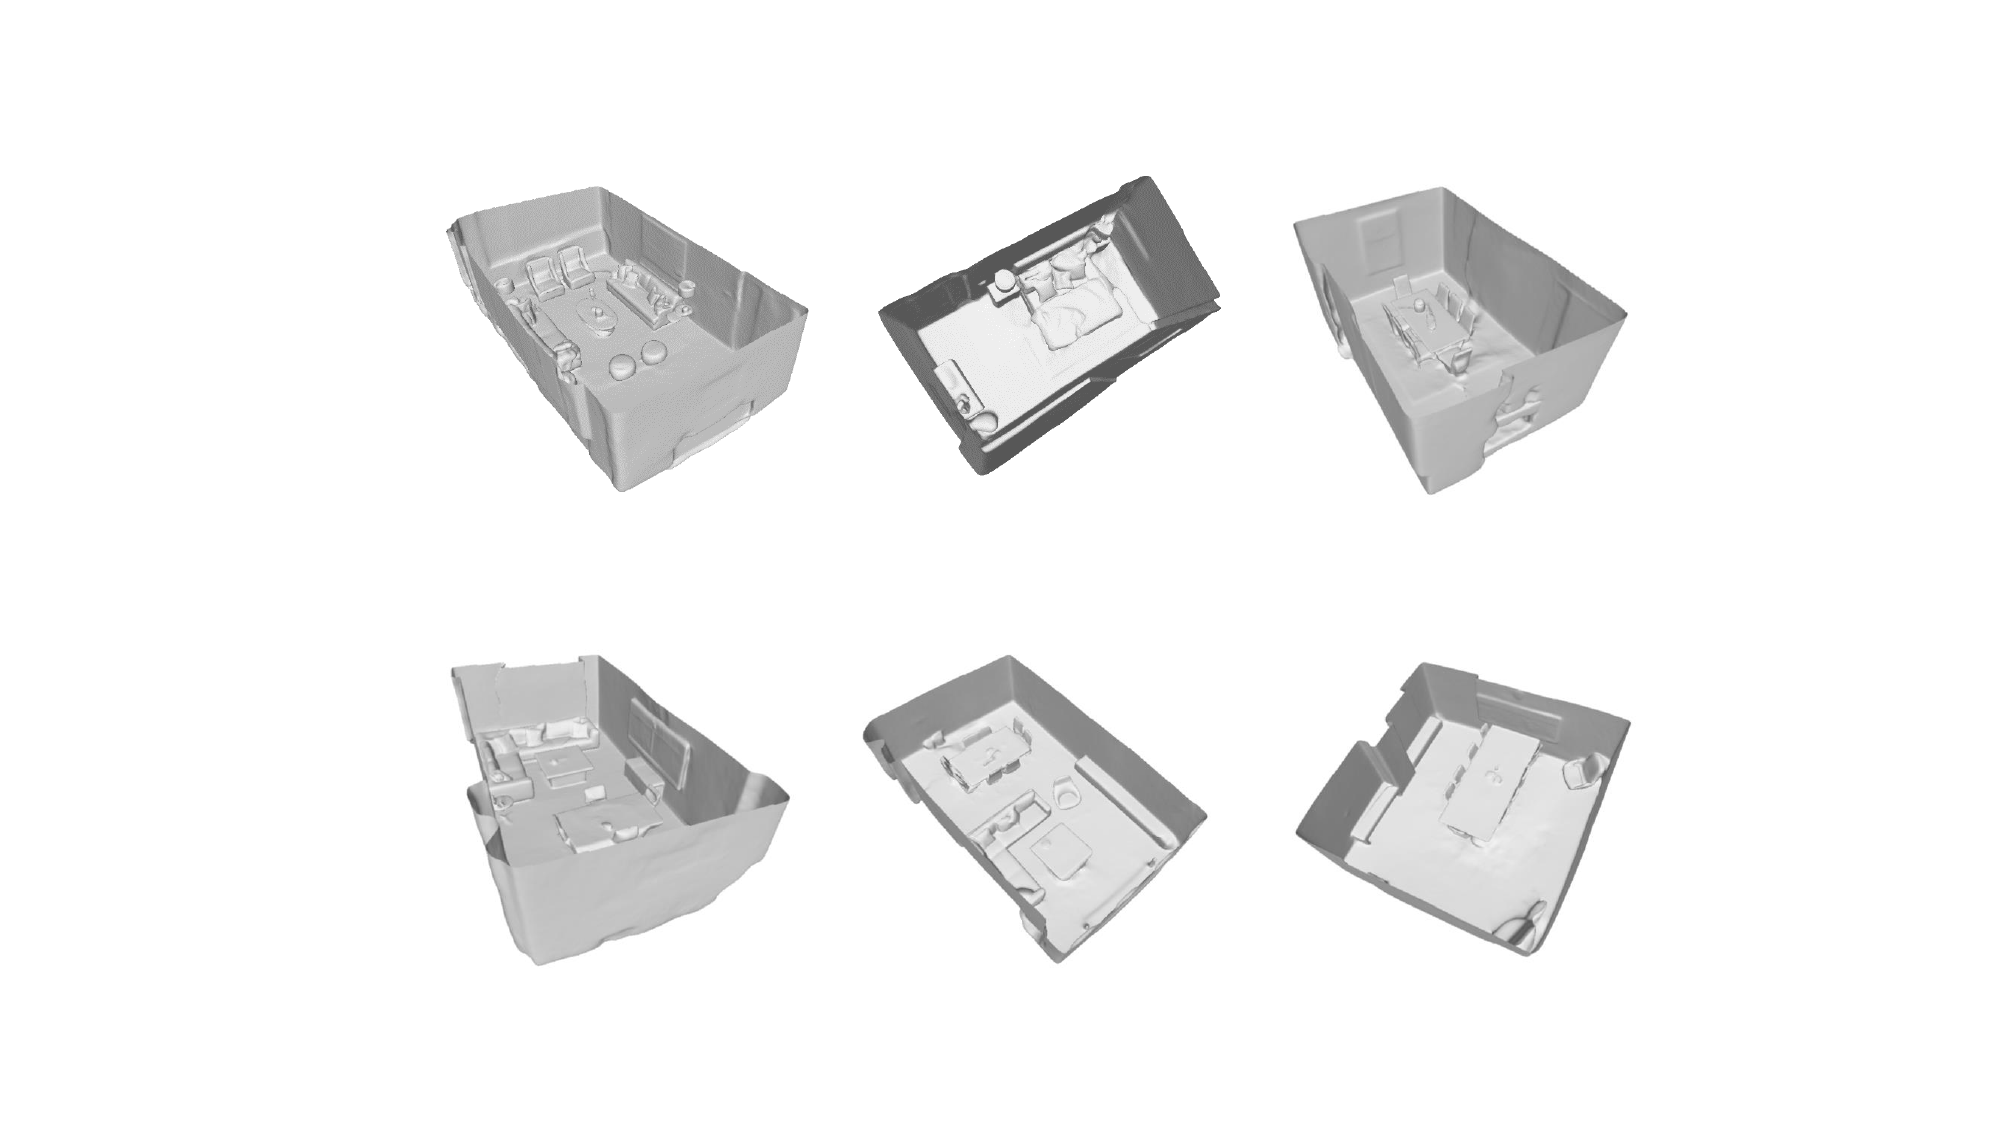}};
        \node[font=\large] at (-4,0.25) {(a)};
        \node[font=\large] at (0.5,0.25) {(b)};
        \node[font=\large] at (5,0.25) {(c)};
        \node[font=\large] at (-4,-4.7) {(d)};
        \node[font=\large] at (0.5,-4.7) {(e)};
        \node[font=\large] at (5,-4.7) {(f)};
    \end{tikzpicture}
    \caption{Qualitative Visualization on Replica Dataset}
    \label{fig:supple_replica}
\end{figure}
