# Supplementary material for: H2O-SDF: Two-phase Learning for 3D Indoor Reconstruction using Object Surface Fields
Source: arXiv:2402.08138 source file (2024-03-08)
Supplement: Supplementary file 5 [file Supple_7scenes.tex]

%% Table for common comments.
% 7-scenes
\begin{table}[h!]
\centering
\small
\begin{tabular}{c|cccccc}
\Xhline{3\arrayrulewidth}
\\ [-0.8em]
Model & Accu.$\downarrow$ & Comp.$\downarrow$ & Prec.$\uparrow$ & Recall$\uparrow$ & F-score$\uparrow$ \\ 
\hline
\\ [-0.8em]
ManhattanSDF & \textbf{0.112} & 0.132 & 0.351 & 0.326 & 0.336 \\
\\ [-0.9em]
NeuRIS & 0.133 & 0.132 & 0.405 & 0.424 & 0.410 \\
\\ [-0.9em]
MonoSDF &0.158	&0.328	&0.286	&0.262	&0.301\\
\\ [-0.9em]
\hline
\\ [-0.9em]
$\text{H}_2\text{O-SDF}$ & 0.128 & \textbf{0.129} & \textbf{0.416} & \textbf{0.469} & \textbf{0.447}
\\ 
\Xhline{3\arrayrulewidth}
\end{tabular}
\caption{Comparison results for 7-Scenes}
\label{tab:sup_7scenes}
\end{table}

% \begin{table}[h]
% \centering
% \small
% \begin{tabular}{M{3.0cm}| M{1.1cm} M{1.1cm} M{1.1cm} M{1.1cm} M{1.1cm}}
% \Xhline{3\arrayrulewidth}
% \\ [-0.5em]
% Methods & Accu.$\downarrow$ & Comp.$\downarrow$ & Prec.$\uparrow$ & Recall$\uparrow$ & F-score$\uparrow$
% \\ [0.5em]
% \Xhline{0.3\arrayrulewidth}
% \\ [-0.8em]
% ManhattanSDF & 0.112 & 0.132 & 0.351 & 0.326 & 0.336 \\
% \\ [0.2em]
% \\ [-0.8em]
% NeuRIS & 0.133 & 0.132 & 0.405 & 0.424 & 0.410 \\
% \\ [0.2em]
% \\ [-0.8em]
% MonoSDF & 0.112 & 0.132 & 0.351 & 0.326 & 0.336 \\
% \\ [0.2em]

% \Xhline{0.3\arrayrulewidth}
% \\ [-0.8em]
% \textbf{$\text{H}_2\text{O-SDF}$} & \textbf{0.128} & \textbf{0.129} & \textbf{0.416} & \textbf{0.469} & \textbf{0.447} 
% \\ [0.2em]
% \Xhline{2\arrayrulewidth}
% \end{tabular}
% \caption{Comparison results for 7-Scenes}
% \label{tab:7scenes}
% \end{table}
