# Supplementary material for: H2O-SDF: Two-phase Learning for 3D Indoor Reconstruction using Object Surface Fields
Source: arXiv:2402.08138 source file (2024-03-08)
Supplement: Supplementary file 7 [file Supple_replica.tex]

\begin{table}[h!]
\centering
\small
\begin{tabular}{c|cccccc}
\Xhline{3\arrayrulewidth}
\\ [-0.8em]
Model & Accu.$\downarrow$ & Comp.$\downarrow$ & Prec.$\uparrow$ & Recall$\uparrow$ & F-score$\uparrow$ \\ 
\hline
\\ [-0.8em]
ManhattanSDF & 0.131 & 0.417 & 0.644 & 0.407 & 0.492 \\
\\ [-0.8em]
NeuRIS & 0.023 & 0.027 & 0.921 & 0.898 & 0.909 \\
\\ [-0.8em]
MonoSDF & 0.020 & 0.017 & 0.951 & 0.923 & 0.934 \\
\\ [-0.8em]
\hline
\\ [-0.8em]
$\text{H}_2\text{O-SDF}$ & \textbf{0.016} & \textbf{0.025} & \textbf{0.983} & \textbf{0.935} & \textbf{0.957} \\ 
\Xhline{3\arrayrulewidth}
\end{tabular}
\caption{Comparison results for Replica}
\label{tab:sup_replica}
\end{table}
